# Supplementary material for: An Efficient Hash-based Data Structure for Dynamic Vision Sensors and its Application to Low-energy Low-memory Noise Filtering
Source: arXiv:2304.14688 source file (2023-04-28)
Supplement: Supplementary file 1 [file Appendix.tex]

\appendix
\label{Appendix}
%\section*{Appendix}\label{Appendix}
\subsection{Derivation of F1 Theoretical prediction equation} \label{F1_Theoretical}
Predicted values of the False Positive Rate ($FPR$) and False Negative Rate ($FNR$) can be combined to predict the F1 score; the optimum memory configuration (FIFO width, depth) for maximizing the F1 score for a given memory size can be determined using sample event data from a given dataset.
\begin{comment}
\setlength{\abovedisplayskip}{0.5em}
\setlength{\belowdisplayskip}{0.5em}
\setlength{\abovedisplayshortskip}{0.5em}
\setlength{\belowdisplayshortskip}{0.5em}
\begin{equation}
\label{eqn:F1_sup}
F1 = \frac{2 {\cdot} p {\cdot} r}{p+r}
\end{equation}
%
where $p$ is the Precision and $r$ is the Recall, defined as:
\begin{equation}
\label{eqn:pr_sup}
p = \frac{TP}{TP+FP}; \; r = \frac{TP}{TP+FN}
\end{equation}
\end{comment}
%
$TP$, $FP$, $TN$, $FN$ are the number of True Positives, False Positives, True Negatives and False Negatives in the sample respectively.
Substituting for precision and recall in the equation for F1 score and simplifying:
\begin{equation}
\label{eqn:F1_sup1}
F1 = \frac{2 \cdot TP}{2 {\cdot} TP + FP + FN}
\end{equation}
 $FPR$ and $FNR$ are defined as:
\begin{equation}
\label{eqn:FPR_FNR_sup}
FPR = \frac{FP}{N_N}; \; FNR = \frac{FN}{N_P}
\end{equation}
where $N_P$ is the number of signal events in the sample and $N_N$, the number of noise events in the sample.
\begin{equation}
\label{eqn:P_sup}
N_P = TP+FN; \; N_N = FP+TN
\end{equation}
From (\ref{eqn:FPR_FNR_sup}),
\begin{equation}
\label {eqn:FP_FN_sup}
FP = N_N {\cdot} FPR; \; FN = N_P {\cdot} FNR
\end{equation}
From (\ref{eqn:P_sup}) and (\ref{eqn:FP_FN_sup}),
\begin{equation}
\label {eqn:TP_sup}
TP = N_P - FN = N_P {\cdot} (1-FNR)
\end{equation}

Substituting (\ref{eqn:TP_sup}) and (\ref{eqn:FP_FN_sup}) in (\ref{eqn:F1_sup1}),
\begin{equation}
\label{eqn:F1_sup2}
F1 =\frac{2 {\cdot} N_P {\cdot} (1-\langle FNR \rangle)} {N_P {\cdot}  (2 - \langle FNR \rangle) + N_N {\cdot} \langle FPR \rangle}
\end{equation}
%
\begin{comment}
Substituting with the theoretically predicted $FNR$ ($FNR_{Th}$) and theoretically predicted $FPR$ ($FPR_{Th}$) from Section \ref{Proposed Filter} in \ref{eqn:F1_sup2}, we get the equation for the theoretically predicted $F1$ ($F1_{Th}$):
%
%
\begin{equation}
\label{eqn:F1_th_sup}
F1_{Th} =\frac{2 {\cdot} N_P {\cdot} (1-FNR_{Th})}{N_P {\cdot}  (2 - FNR_{Th}) + N_N {\cdot} FPR_{Th}}
\end{equation}
\end{comment}
%
%
\subsection{Hardware implementation of hash functions---comparison of area and power}\label{hash_comparison}
We performed logic synthesis targeting the TSMC 40nM process using both the H$_3$ hash function \cite{Ramakrishna1994} used in our hardware implementation and the LSH hash function used in  \cite{Guo2021}. Both the functions were coded in Verilog. A comparison of the resource requirements and power consumption of the two hash functions is given in Table \ref{tab:hash_comparison}; it can be seen that the H$_3$ function has a clear advantage with respect to both these measures.
\begin{table}[htbp]
\centering
\caption{Hash functions - logic synthesis results}
\label{tab:hash_comparison}
\begin{tabular}{|l|r|r|}
\hline
\multicolumn{1}{|c|}{\textbf{Hashing Function}} & \multicolumn{1}{c|}{\textbf{Area}} & \multicolumn{1}{c|}{\textbf{\begin{tabular}[c]{@{}c@{}}Power (nW)\\ (Clock = 1 Mhz)\end{tabular}}} \\ \hline
\begin{tabular}[c]{@{}l@{}}LSH (HashHeat)\\ (Sensor = $1280 \times 960$,\\  FIFO width = 4096)\end{tabular} & 3274 & 26370 \\ \hline
\begin{tabular}[c]{@{}l@{}}H$_3$ (Our work)\\ (Sensor = $1280 \times 960$,\\ FIFO width = 65536)\end{tabular} & 104 & 766 \\ \hline
\end{tabular}
\end{table}

\subsection {\textit{Energy (pJ) per event calculations for different filters (Table \ref{tab:pJ_per_event})}}

\href{https://sites.google.com/d/1_OgA3afkYty_kwO8YGwz_m8j0U1XJXU4/p/1jFRfzFOoBVy-B4efXFTcqzANnVVMWE0j/edit} {\textcolor{blue}{Link to website}}

\subsection {\textit{ Calculation of energy (pJ) per event and Memory requirement of BAF} used to create fig. \ref{fig:baf_pj_mem}}

\href{https://sites.google.com/d/1_OgA3afkYty_kwO8YGwz_m8j0U1XJXU4/p/1jFRfzFOoBVy-B4efXFTcqzANnVVMWE0j/edit} {\textcolor{blue}{Link to website}}
